# Supplementary material for: DropoutGS: Dropping Out Gaussians for Better Sparse-view Rendering
Source: arXiv:2504.09491 source file (2025-04-13)
Supplement: Supplementary file 1 [file X_suppl.tex]

\clearpage
\setcounter{page}{1}
% 修改章节编号格式为大写罗马数字

\maketitlesupplementary
\appendix

\section*{Overview}
\label{sec:supp-Overview}
In the supplementary materials, we discuss the additional results, experiment details, and the limitations of our work. In Sec.~\ref{sec:supp-addition_results}, we report the additional results of the performance evaluation (Sec.~4.2 of the main paper). In Sec.~\ref{sec:supp-details}, we provide more details about our experiment settings. Finally, we discuss the limitations of our method in  Sec.~\ref{sec:supp-limitation}.

\section{Additional Results}
\label{sec:supp-addition_results}
We provide more visualization results including RGB images and depth maps from DropoutGS with 3 views as input on the DTU in Fig.~\ref{img:additional_dtu}. Compared with DNGaussian, our DropoutGS can capture more accurate 3D characteristics and render clean novel views. We also show the rendering results of DropoutGS in the more view setting in Fig.~\ref{img:additional_llff}. Figure~\ref{img:additional_compatibility} illustrates the performance of other 3DGS-based methods with and without our approach. 
\begin{figure*}[t]
    \centering
    \includegraphics[width=\linewidth]{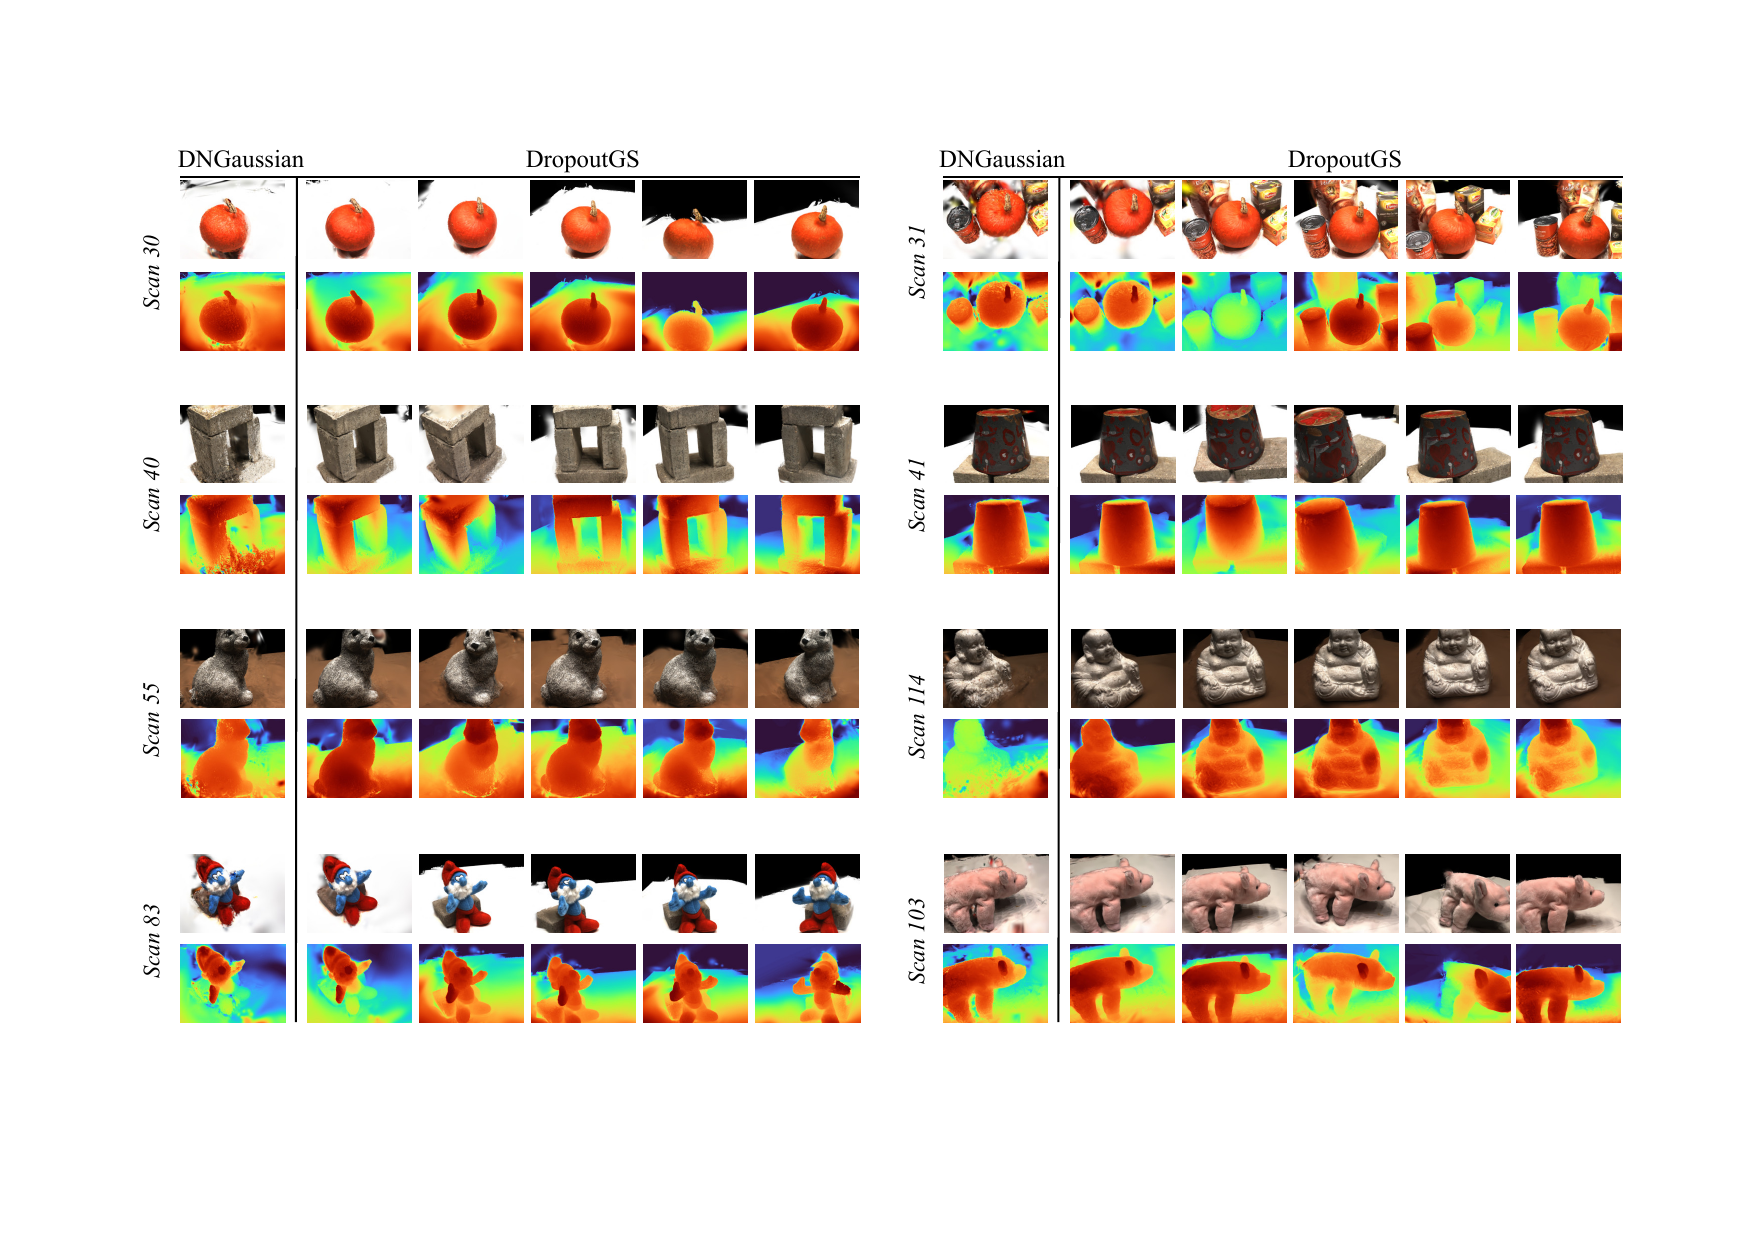}
    \caption{\textbf{Additional novel views and depth maps rendered from DropoutGS with 3 views on the DTU dataset.} }
    \label{img:additional_dtu}
    \vspace{0.5cm}
\end{figure*}
\begin{figure*}[t]
    \centering
	\begin{minipage}{\linewidth}
		\centering
        \subfloat[3 views]{\includegraphics[width=\linewidth]{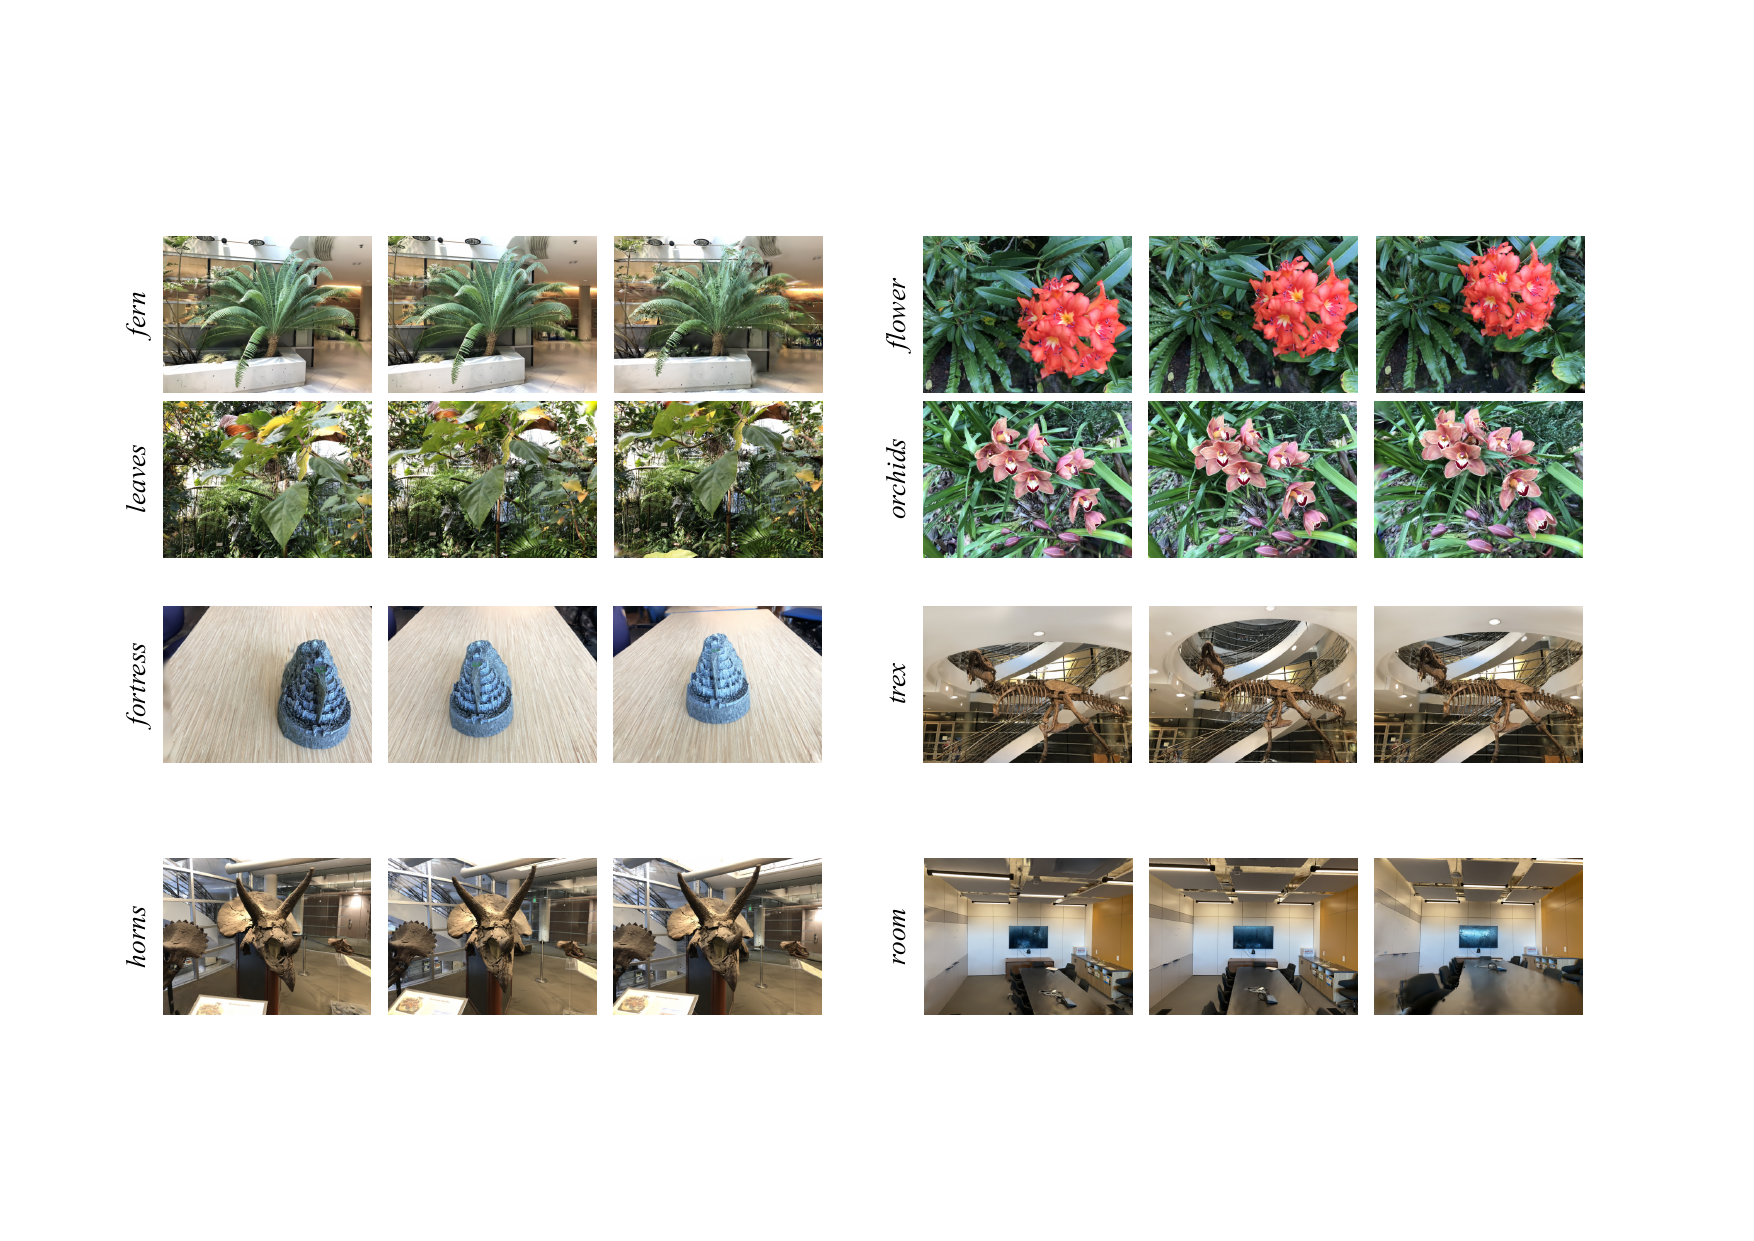}}
	\end{minipage}\\
	% \vspace{.2cm}
	\begin{minipage}{\linewidth}
		\centering
		\subfloat[6 views]{\includegraphics[width=\linewidth]{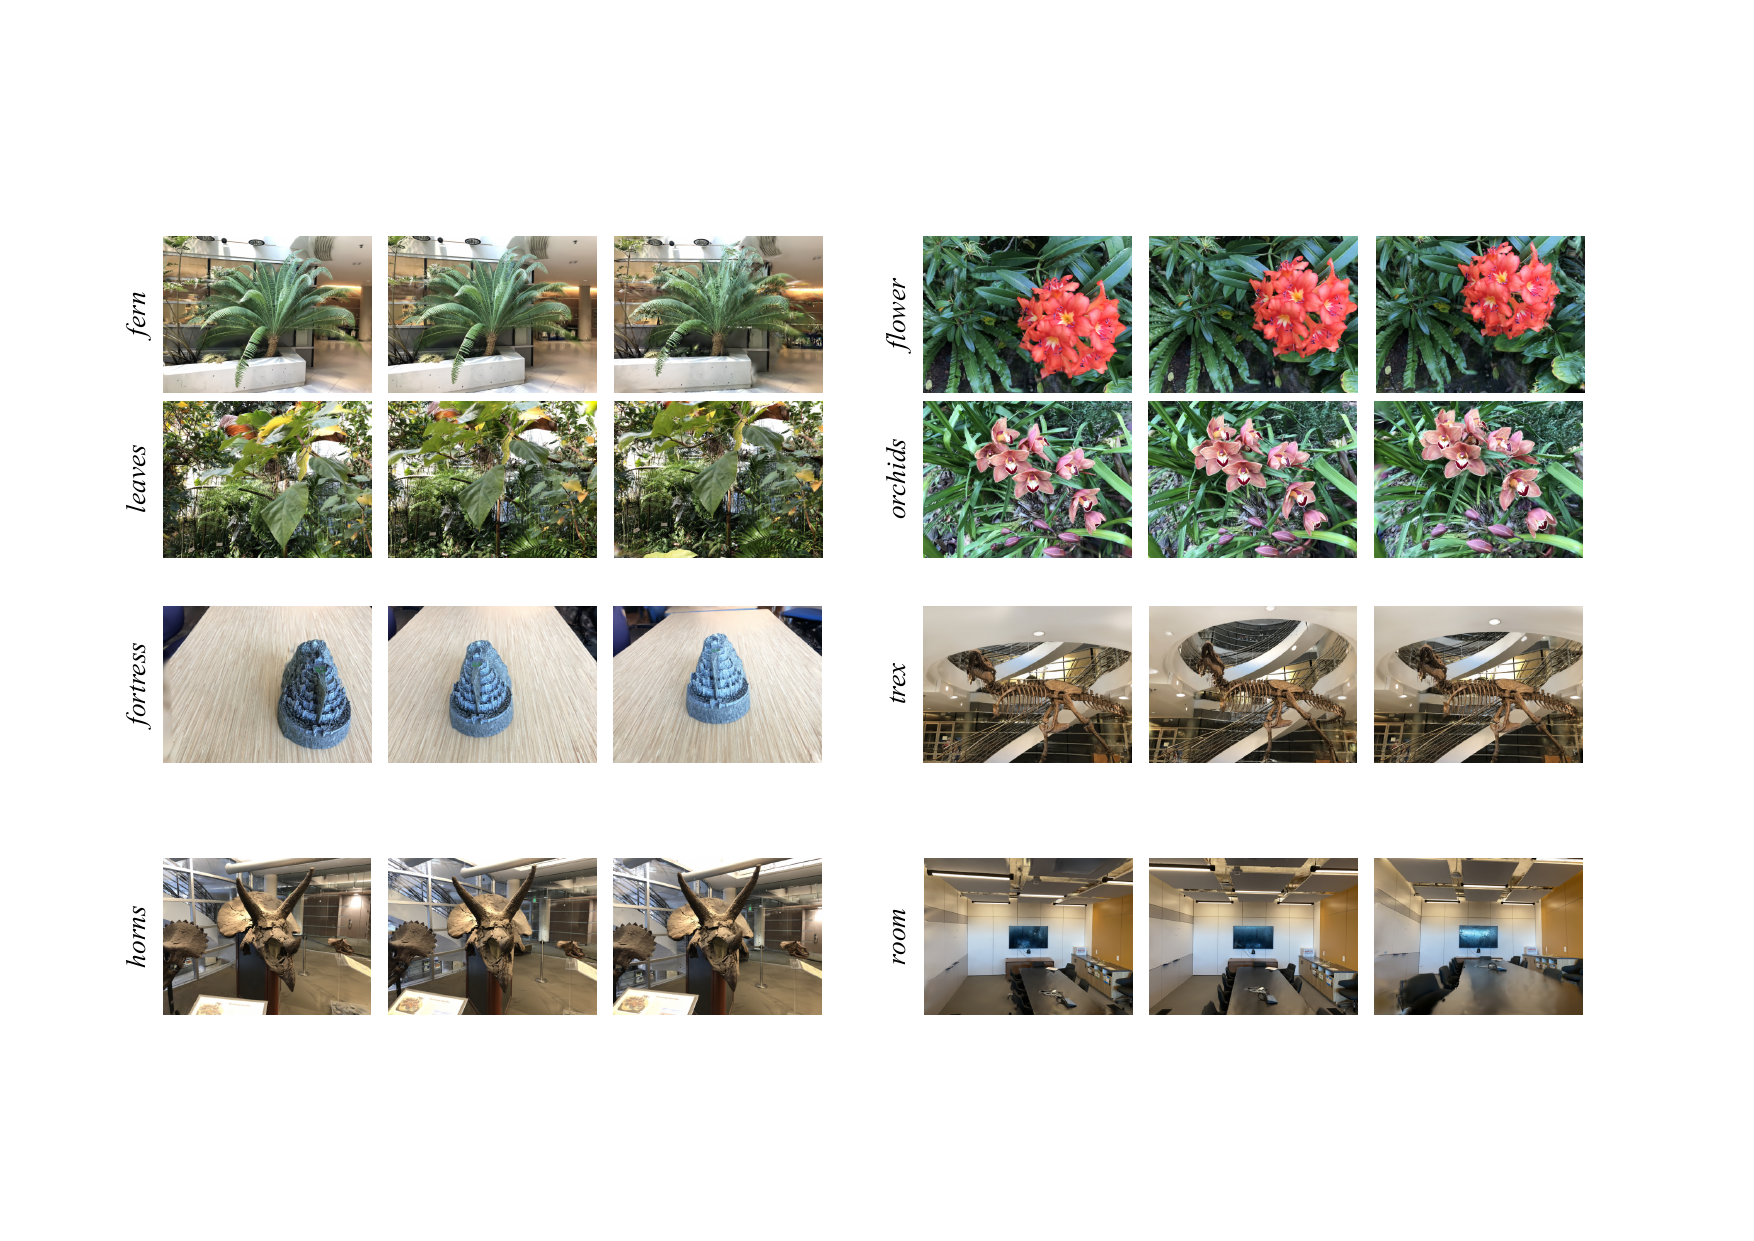}}
	\end{minipage}\\
         % \vspace{.2cm}
 	\begin{minipage}{\linewidth}
		\centering
        \subfloat[9 views]{\includegraphics[width=\linewidth]{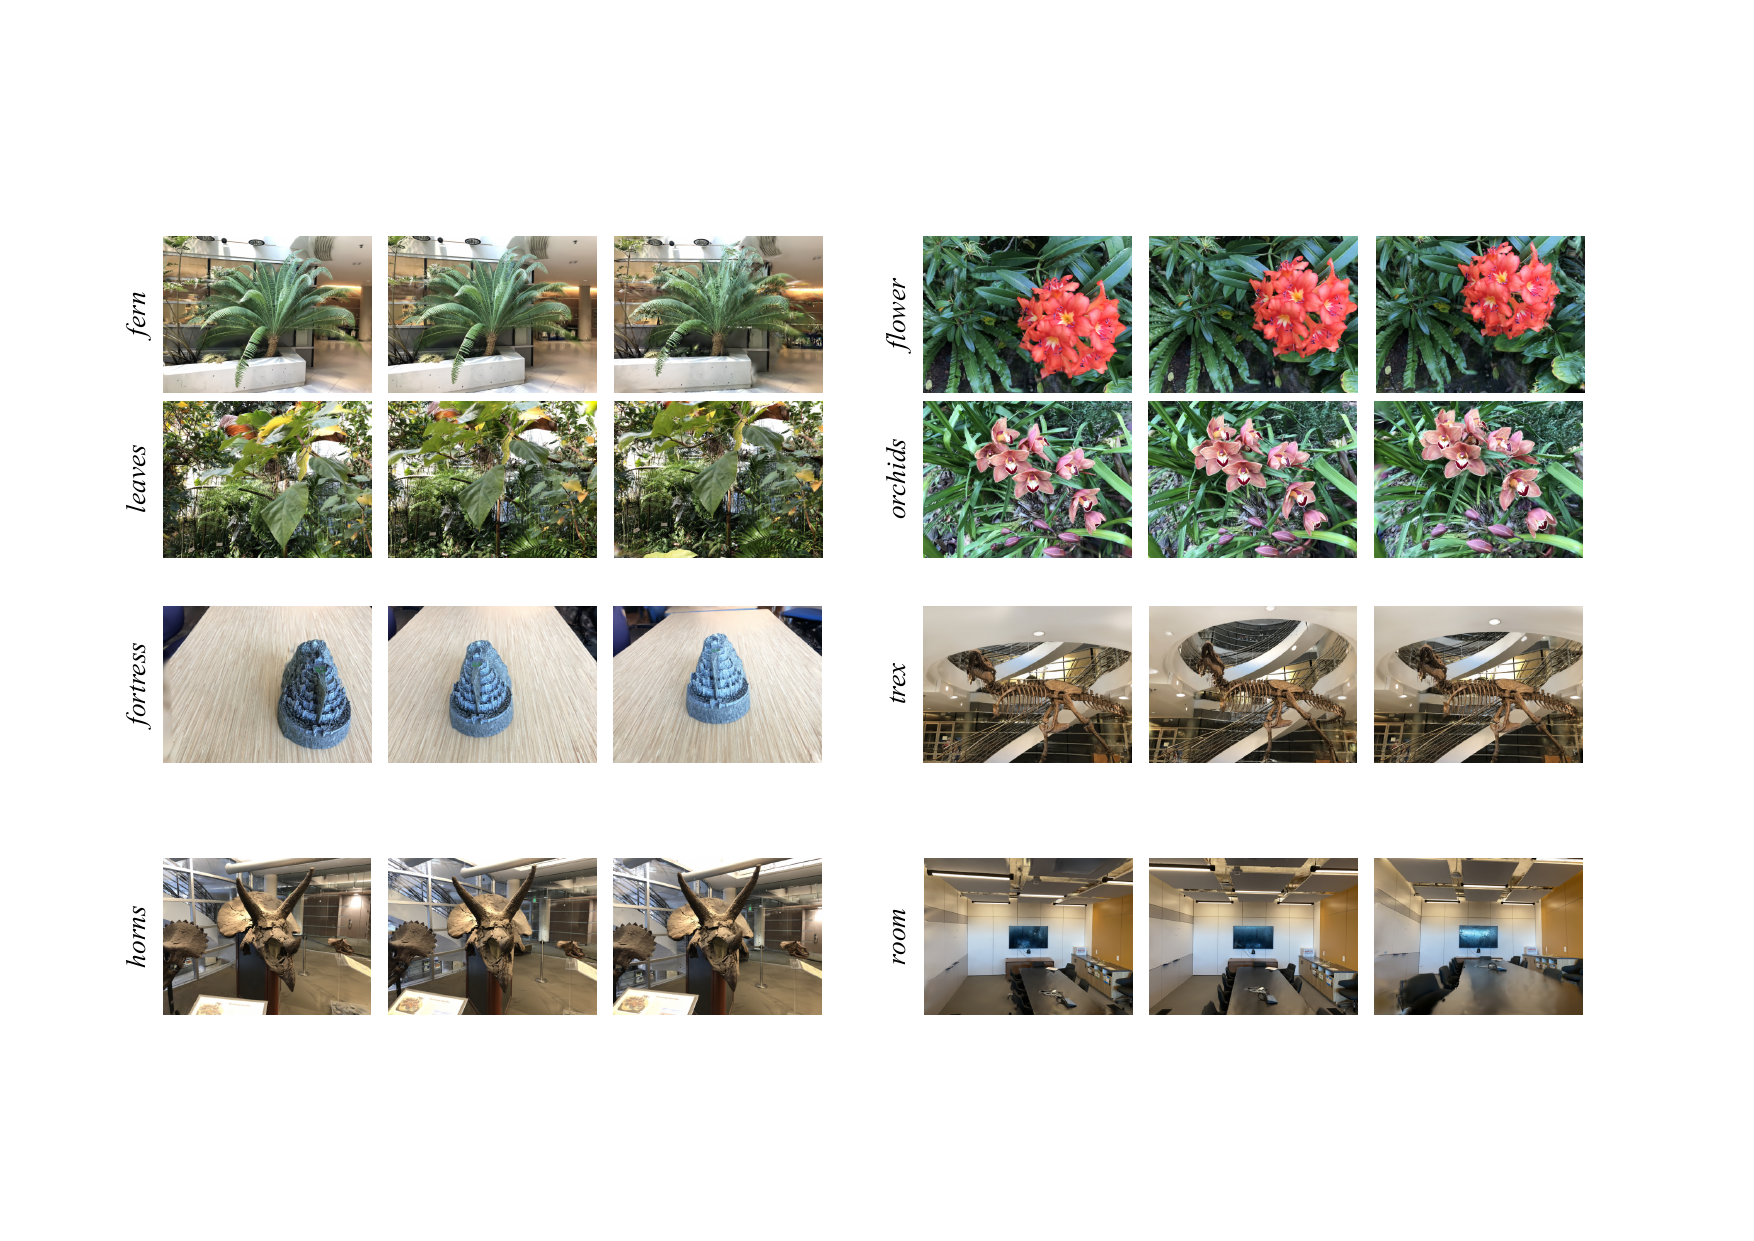}}
	\end{minipage}\\
    \caption{\textbf{Additional novel views synthesis results from DropoutGS using 3, 6, and 9 views as input on the LLFF dataset.} }
        \label{img:additional_llff}
    % \vspace{-.8cm}
\end{figure*}
\begin{figure*}[t]
    \centering
    \includegraphics[width=0.90\linewidth]{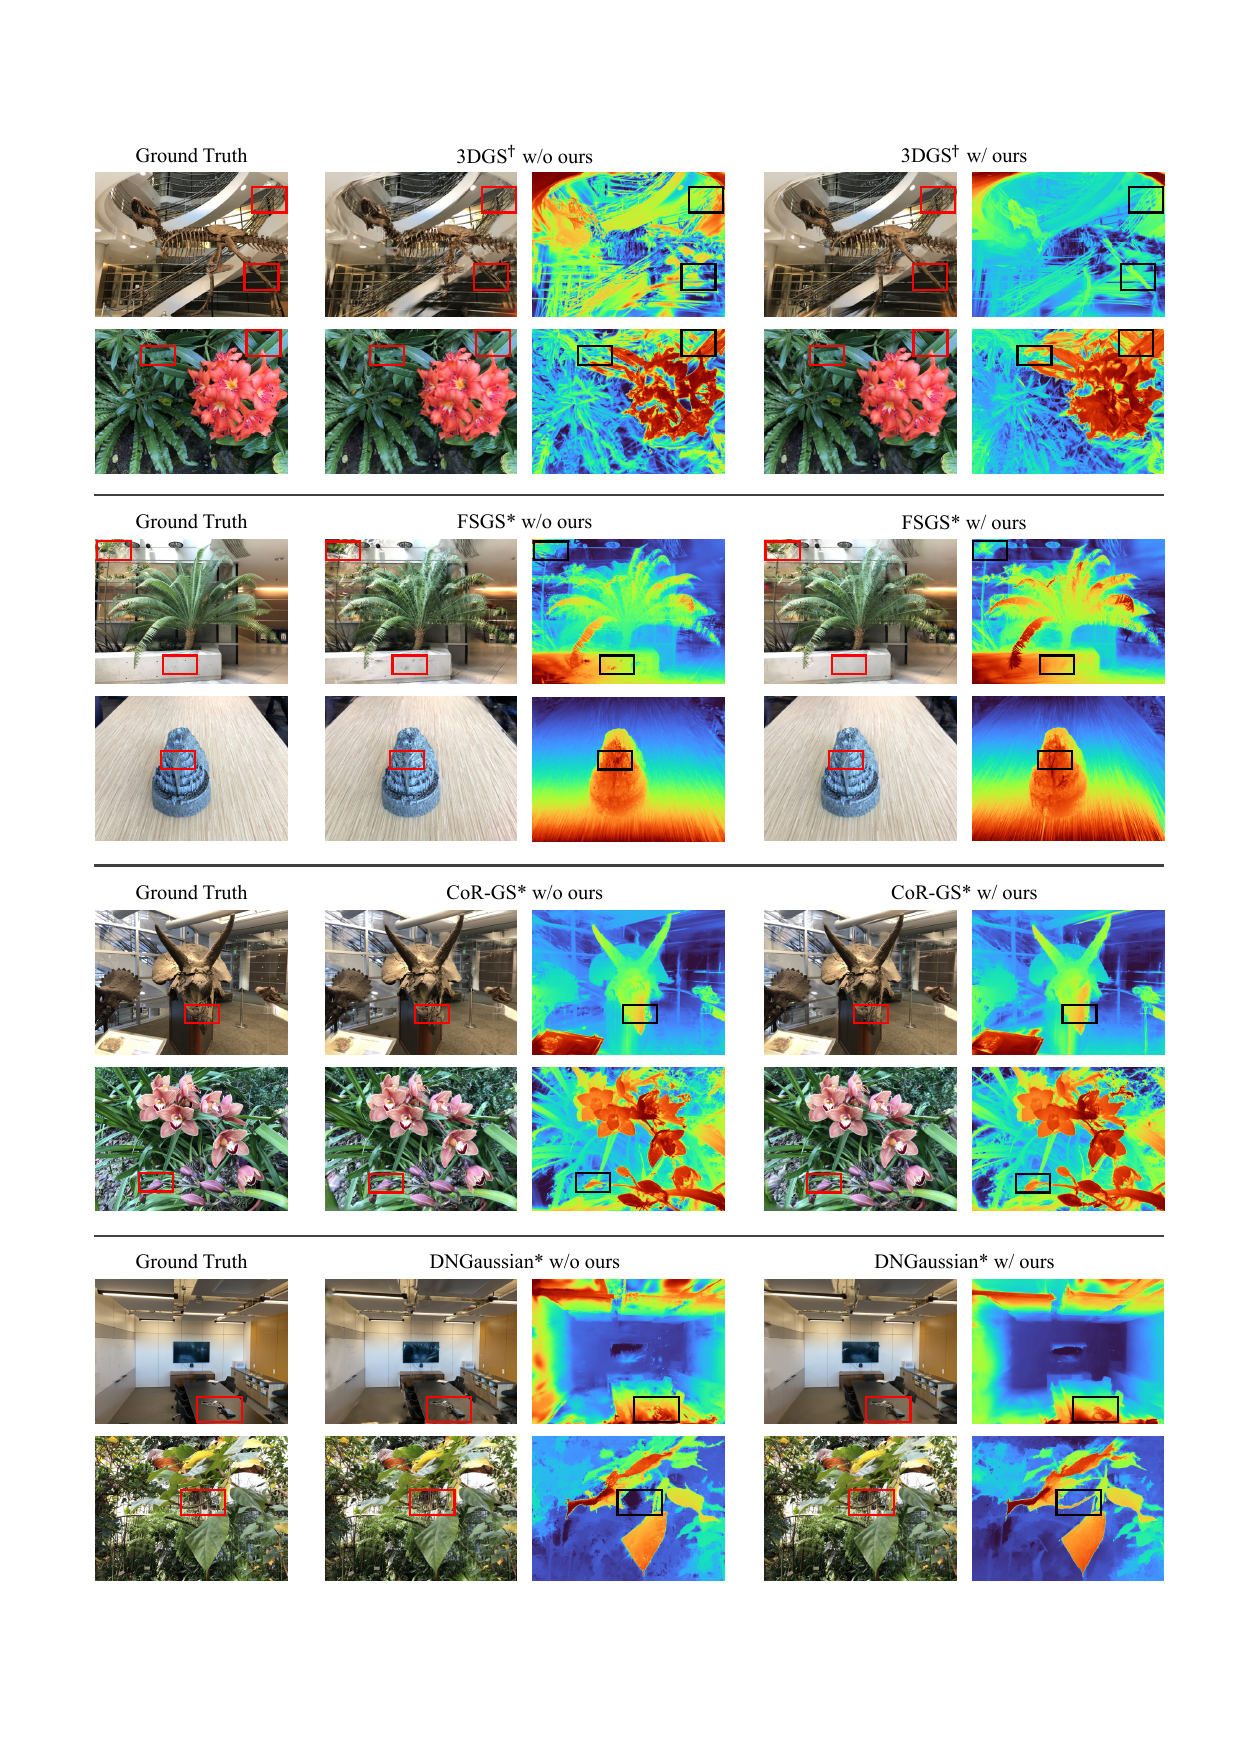}
    \caption{\textbf{Additional rendered images and depth maps of the compatibility experiments on the LLFF dataset.} * with MVS point cloud as initialization. \small\dag \ with the same hyperparameters and the neural color renderer as DNGaussian.}
    \label{img:additional_compatibility}
    % \vspace{1cm}
\end{figure*}

% \vspace{-0.15cm}
\section{Experimental Details}
\label{sec:supp-details}
\subsection{Implementations}
\vspace{2pt}\noindent\textbf{DropoutGS.} We use the pre-trained DPT estimator \cite{DPT} to generate monocular depth maps for geometry regularization, following the approach in \cite{DNGS}. For the LLFF dataset, we adopt the $\textit{dpt\_hybrid\_384}$ model, while the $\textit{dpt\_large\_384}$ model is used for DTU and Blender. Additionally, we employ a neural color renderer to predict colors for each Gaussian, replacing spherical harmonics, as in DNGaussian, to achieve high-quality rendering. We conduct the experiments with a single GeForce RTX 3090 and the average training time is around 3 minutes per scene with 6k iterations. 

\vspace{2pt}\noindent\textbf{Random Dropout Regularization.}
The dropout rate is set to 0.4 on the LLFF dataset and 0.3 on the DTU dataset. For the regularization coefficient $\lambda_{RDR}$, it is set to 0.2 for LLFF and 0.5 for DTU.

\vspace{2pt}\noindent\textbf{Edge-Guided Splatting Strategy.}
We employ the Sobel Edge Detector \cite{castleman1996digital} to obtain the edge maps for edge score calculation. The edge threshold is set to $1\times10^{-3}$ and $5\times10^{-2}$ for LLFF and DTU, respectively. The scale threshold is set to 50 and 1 times of the size threshold used in the original splitting on the LLFF and DTU datasets, respectively.

\subsection{Dataset}
\vspace{2pt}\noindent\textbf{LLFF.}
The LLFF dataset contains 8 challenging forward-facing scenes. Following \cite{DNGS, FreeNeRF}, we use every 8 images as the test set while evenly sampling among the remaining images as the training set. In practice, we downsample the original images 8 times to the resolution of $378\times504$.

\vspace{2pt}\noindent\textbf{DTU.}
We evaluate our method on 15 out of the total 124 object-centered scenes included in the DTU dataset following the previous works \cite{DNGS, FreeNeRF}. The scan IDs of the test scenes are 8, 21, 30, 31, 34, 38, 40, 41, 45, 55, 63, 82, 103, 110, and 114. In each scene, we use the images with the IDs 25, 22, and 28 as the input views while the IDs 1,
2, 9, 10, 11, 12, 14, 15, 23, 24, 26, 27, 29, 30, 31, 32, 33, 34, 35, 41, 42, 43, 45, 46 and 47 as evaluation views. The image size is downsampled 4$\times$ in the implementation. 

\vspace{2pt}\noindent\textbf{Blender.}
Blender contains 8 synthetic scenes, each providing viewpoints covering 360 degrees. We follow the data split used in previous works \cite{FreeNeRF, DietNeRF} and take the selected 8 views as input with IDs 26, 86, 2, 55, 75, 93, 16, 73, and 8. The 25 test views are evenly sampled from the testing set for evaluation. We downsample all images to the resolution of $400\times 400$ during the experiments.

\section{Limitation}
\label{sec:supp-limitation}
DropoutGS introduces dropout into sparse 3DGS to alleviate overfitting degradation with limited inputs, achieving significant improvement in the rendering quality. However, our approach still has the following limitations. 1) Dropout rate and edge threshold are critical to the final performance and require careful tuning per scene to obtain optimal results. 2) Our method introduces large improvements to methods initialized with random point clouds while the gains are weakened for well-initialized Gaussians.
